# Supplementary material for: Theoretical Validation of Potential Habitability via Analytical and Boosted Tree Methods: An Optimistic Study on Recently Discovered Exoplanets
Source: arXiv:1712.01040 ancillary file (2017-12-04)
Supplement: Supplementary file 1 [file supplementary-file.pdf]

# Supplementary file to the manuscript "Theoretical validation of potential habitability via analytical and boosted tree methods: An optimistic study on recently discovered exoplanets"

Snehanshu Saha, Suryoday Basak, Margarita Safonova, Kakoli Bora,
Surbhi Agrawal, Poulami Sarkar and Jayant Murthy

## 1 A theoretical framework for missing value imputation: Surface Temperature: Context of the Problem

In the PHL-EC, eleven rocky planets (Table 1), do not have their surface temperature provided, which creates the problem of missing values. We tackle the missing values with the help of attribute mining and association rules.

Table 1: Rocky planets with unknown surface temperature: **Association Rule Mining** – *Oversampling, attribute mining for missing value imputation (surface temperature)*

| *P.Name* | *P.Composition Class* |
|---|---|
| Kepler-132 e | rocky-iron |
| Kepler-157 d | rocky-iron |
| Kepler-166 d | rocky-iron |
| Kepler-176 e | rocky-iron |
| Kepler-192 d | rocky-iron |
| Kepler-217 d | rocky-iron |
| Kepler-271 d | rocky-iron |
| Kepler-398 d | rocky-iron |
| Kepler-401 d | rocky-iron |
| Kepler-403 d | rocky-iron |
| WD 1145+017 b | rocky-iron |

Table 2: Table of features used to construct the association rule for missing value imputation

| *P.Name* | *P.Zone Class* | *P.Mass Class* | *P.Composition Class* | *P.Atmosphere Class* | Class Label |
|---|---|---|---|---|---|
| 8 Umi b | Hot | Jovian | gas | hydrogen-rich | non-habitable |
| GJ 163 c | Warm | Superterran | rocky-iron | metals-rich | psychroplanet |
| GJ 180 b | Warm | Superterran | rocky-iron | metals-rich | mesoplanet |
| GJ 180 c | Warm | Superterran | rocky-iron | metals-rich | mesoplanet |
| 14 Her b | Cold | Jovian | gas | hydrogen-rich | non-habitable |

There are missing values of surface temperature of exoplanets listed in Table 1. The values of equilibrium temperature of those entries are also unknown. Imputation of missing values is commonly done by filling in the blanks by computing the mean of continuous valued variables in the same column, using other entries of the same type, rocky planets in this case. However, this method has demerits. We propose the following method to achieve the task of imputing missing surface temperature values.

## 2 Data Imputation Using Association Rules

A more sophisticated method of data imputation is that of *rule-based learning*. Popularized by Agrawal et al. through their seminal paper in 1993, it is a robust approach in Data Mining and Big Data Analytics for the pur-

pose of filling in missing values. The original approach was inspired by unexpected correlations in items being purchased by customers in markets. An illustrative example making use of samples and features from the PHL-EC dataset is presented here.

Any dataset has samples and features. Say, we have n samples $S = \{s_1, s_2, ..., s_n\}$ and $m$ features, $X = \{X_1, X_2, ..., X_m\}$, such that each sample is considered to be a $1 \times m$ vector of features, $s_i = \{x_{i1}, x_{i2}, ..., x_{im}\}$. Here, we would like to find out if the presence of any feature set $A$ amongst all the samples in $S$ implies the presence of a feature set $B$.

Consider Table 2. An interesting observation is that all the planets with *P.Zone Class = Warm, P.Mass Class = Superterrain* and *P. Composition Class = rocky-iron* (the planets GJ 163 c, GJ 180 b and GJ 180 c) also have *P. Atmosphere Class* as *metals-rich*. Here, if we consider conditions $A = \{$*P.Zone Class = Warm, P.Mass Class = Superterran, P.Composition Class = rocky-iron*$\}$ and $B = \{$*P.Atmosphere Class = metals-rich*$\}$, then $A \Rightarrow B$ holds true. But what does it mean in for data imputation? If there exists a sample $s_k$ in the dataset such that condition A holds good for $s_k$ but the value of *P.Atmosphere Class* is missing, then by the association rule $A \Rightarrow B$, we can impute the value of *P.Atmosphere Class* for $s_k$ as metals rich. Similarly, if $A' = \{$*P.Mass Class = Jovian, P.Composition Class = gas*$\}$ and $B' = \{$*P.Atmosphere Class = hydrogen-rich*$\}$, then $A' \Rightarrow B'$ becomes another association rule which may be used to impute vales of *P.Atmosphere Class*. Note here the exclusion of the variable *P.Zone Class*. In the two samples which satisfy $A'$, the value of *P.Zone Class* are not the same and hence they do not make for a strong association with $B'$.[1]

In Table 2, we have mentioned the class labels alongside the samples. However this is just indicative; the class labels should not be used to form associations (if they are used, then some resulting associations might become similar to a traditional classification problem!) Different metrics are used to judge how interesting a rule is, i.e., the goodness of a rule. Two of the fundamental metrics are:

1. **Support**: It is an indicator of how frequently a condition A appears in the database. Here, $t$ is the set of samples in $S$ which exhibit the condition $A$.

$$supp(A) = \frac{|t \in S; A \subseteq t|}{|S|}. \quad (1)$$

In the example considered, $A = \{$*P.Zone Class = Warm, P.Mass Class = Superterran, P.Composition Class = rocky-iron*$\}$ has a support of $3/5 = 0.6$.

2. **Confidence**: It is an indication of how often the rule was found to be true. For the rule $A \Rightarrow B$ in S, the confidence is defined as:

$$conf(A \Rightarrow B) = \frac{supp(A \cup B)}{supp(A)}. \quad (2)$$

For example, the rule $A \Rightarrow B$ considered in our example has a confidence of $0.6/0.6 = 1$, which means 100% of the samples satisfying $A = \{$*P.Zone Class = Warm, P.Mass Class = Superterran, P.Composition Class = rocky-iron*$\}$ will also satisfy $B = \{$*P.Atmosphere Class = metals-rich*$\}$.

Association rules must satisfy thresholds set for support and confidence in order to be accepted as rules for data imputation. The example illustrated is a very simple one. In practice, association rules need to be considered over thousands or millions of samples. From one dataset, millions of association rules may arise. Hence, the support and confidence thresholds must be carefully considered. The example makes use of only categorical variables for the sake of simplicity. However, association rules may be determined for continuous variables by considering bins of values. Algorithms exist that are used for discovering association rules, amongst which *a priori* is the most popular. In the original text, the features considered here are called *items* and each sample is called a *transaction*.

# 3 Proof of model scalability

The truth of an infinite sequence of propositions $S_i$ for $i = 1, 2, ...n$ is established if

[1]Supplementary file to the main paper submitted to IEEE Transactions on ETICI

- $S_1$ is true (a basis step); and
- $S_n$ (induction hypothesis) implies $S_{n+1}$ for all $n$ (an inductive step).

If $S_n$ holds for an arbitrary number of input parameters, the same condition for global maxima shall hold when the number of parameters increases by 1, i.e. $S_{n+1}$. The condition for DRS/CRS/IRS are known for $n$ unknowns previously [1]. Let $S(n)$ be the premise for some natural number $n \in N$. Let us check if $S(1)$ is true.
Let us represent $S(n) = \log(y)$ as the product of two functions, say $f(n)$ and $g(n)$, where,

$$f(n) = \log\left\{k\prod_{i=1}^{n}\left(\frac{x_i p}{w_i}\right)^{\alpha_i}\right\} \tag{3}$$

and

$$\begin{aligned} g(n) &= \sum_{i=1}^{n}\Big(t(n) - t(n-1)\Big) \\ &= \sum_{i=1}^{n}\left(\frac{1}{1-\sum\limits_{i=1}^{n}\alpha_i} - \frac{1}{1-\sum\limits_{i=1}^{n-1}\alpha_i}\right), \end{aligned} \tag{4}$$

where

$$t(n) = \frac{1}{1-\sum\limits_{i=1}^{n}\alpha_i}\,. \tag{5}$$

Clearly, $g(0) = 0$.
**Basis Step: For** $n = 1 : S(1)$

$$\begin{aligned} f(1) &= \log\left\{k\prod_{i=1}^{1}\left(\frac{x_i p}{w_i}\right)^{\alpha_i}\right\} \\ f(1) &= \log\left\{k\left(\frac{x_1 p}{w_1}\right)^{\alpha_i}\right\} \end{aligned} \tag{6}$$

Similarly, we have

$$\begin{aligned} g(1) = t(1) - t(0) &= \sum_{i=1}^{1}\frac{1}{1-\sum\limits_{i=1}^{1}\alpha_i} - 0\,, \\ g(1) &= \frac{1}{1-\alpha_1}\,. \end{aligned} \tag{7}$$

Therefore, $S(1) = f(1).g(1)$,

$$S(1) = \frac{1}{1-\alpha_1}\log\left\{k\left(\frac{x_1 p}{w_1}\right)^{\alpha_i}\right\}\,. \tag{8}$$

This proves that $S(1)$ is true i.e the basis step in the inductive reasoning is validated.

**Induction hypothesis:** Let $S(n)$ be true for an arbitrary $n = m$; Induction Step: NTS, $S(n)$ holds for $n = m+1$ for $f(m+1)$ we have

$$\begin{aligned} f(m+1) &= \log\left\{k\left\{\prod_{i=1}^{m}\left(\frac{x_i p}{w_i}\right)^{\alpha_i}\right\}k\left(\frac{x_{m+1}p}{w_{m+1}}\right)^{\alpha_{m+1}}\right) \\ \Rightarrow (m+1) &= \log\left\{k\prod_{i=1}^{m}\left(\frac{x_i p}{w_i}\right)^{\alpha_i}\right\}\left(k\left(\frac{x_{m+1}p}{w_{m+1}}\right)^{\alpha_{m+1}}\right) \\ \Rightarrow f(m+1) &= \log\left\{k\prod_{i=1}^{m+1}\left(\frac{x_i p}{w_i}\right)^{\alpha_i}\right\}\,. \end{aligned} \tag{9}$$

Similarly, for $g(m+1)$ we have,

$$\begin{aligned}
&g(m+1) = \sum_{i=0}^{m}(t(m) - t(m-1)) + t(m+1) - t(m) \\
&g(m+1) = t(1) - t(0) + t(2) - t(1) + - - - + t(m) \\
&- t(m-1) + t(m+1) - t(m) \\
&g(m+1) = t(m+1) - t(0) \\
&g(m+1) = t(m+1) \\
&g(m+1) = \frac{1}{1 - \sum\limits_{i=1}^{m+1} \alpha_i} \,.
\end{aligned} \tag{10}$$

Since we know that

$$S(m) = f(m).g(m) \tag{11}$$

and

$$S(m+1) = f(m+1).g(m+1)\,, \tag{12}$$

we obtain

$$S(m+1) = \frac{1}{1 - \sum\limits_{i=1}^{m+1} \alpha_i}.f(m+1) = \log\left\{k \prod_{i=1}^{m+1} \left(\frac{x_i p}{w_i}\right)^{\alpha_i}\right\}. \tag{13}$$

This is identical to Equation 3 where $n = m+1$. Thus, we prove that Equation 3 is true for $n = m+1$ whenever it is true for $n = m$. We conclude that the condition for DRS for $n+1$ parameters is true, i.e. $1 - \sum\limits_{i=1}^{m+1} \alpha_i > 0$ is true, if the condition for DRS for $n$ parameters, i.e. $1 - \sum\limits_{i=1}^{m} \alpha_i > 0$ holds, by inductive reasoning.

We describe the algorithm for computing the CDHS of exoplanets by following the method described in Section 2 of the main paper.

**Algorithm 1:** Computing the CDHS of a planet

**Data:** $R$, $D$, $T_s$, $V_e$

**Result:** The habitability class of a planet

1 calculate $\alpha$ and $\beta$ using $SGA(D, R)$;

2 calculate $\gamma$ and $\delta$ using $SGA(T_s, V_e)$;

3 *interior CDHS* is calculated from $D$ and $R$: $CDHS_i = (D)^{\alpha}(R)^{\beta}$;

4 *exterior* or *surface CDHS* is calculated from $T_s$ and $V_e$: $CDHS_s = (T_s)^{\gamma}(V_e)^{\delta}$;

5 convex combination of $CDHS_i$ and $CDHS_s$ gives the final CDHS of a planet by: $CDHS \leftarrow w_1 CDHS_i + w_2 CDHS_s$;

6 return classification result based on CDHS using k-NN with probabilistic herding: $Probabilistic - kNN(CDHS)$;

Next, we describe the algorithm for computing the elasticity, $\alpha$, $\beta$, $\gamma$ and $\delta$, required for CDHS formulation of exoplanets by following the method described in Section 3 of the main paper.

**Algorithm 2:** Stochastic Gradient Ascent

**Data:** $R$,$D$

**Result:** $\alpha$, $\beta$: appropriate exponents of $R$ and $D$ for calculating $CDHS$ of a planet; this is repeated for $T$ and $V_e$ where the corresponding exponents are $\gamma$ and $\delta$ respectively.

choose two initial parameters $\alpha$ and $\beta$ and a randomized learning rate $\Delta$;
$\frac{\partial y}{\partial \alpha} := \alpha R^{\alpha-1} + D^{\beta}$;
$\frac{\partial y}{\partial \beta} := \beta D^{\beta-1} + R^{\alpha}$;
**do**
  $\alpha_{n+1} \leftarrow \alpha_n + \Delta \frac{\partial y}{\partial \alpha}$;
  $\beta_{n+1} \leftarrow \beta_n + \Delta \frac{\partial y}{\partial \beta}$;
  $\alpha_n \leftarrow \alpha_{n+1}$;
  $\beta_n \leftarrow \beta_{n+1}$;
**while** $[(\alpha_{n+1} > 0)||(\beta_{n+1} > 0)||(\alpha + \beta < threshold)]$ *is not satisfied*;

# 4 Algorithm for Habitability candidacy classification

The algorithms described here implement the methods explained in Sections 3 (elasticity computation using stochastic gradient ascent/descent) and 4 (habitability candidate classification) of the main paper. Algorithms 1 and 2 compute the CDHS by calculating the elasticity $\alpha$, $\beta$ and $\gamma$, $\delta$ in pairs. Subsequently, these values and CDHS are used in Algorithm 3 for candidacy class determination.

**Algorithm 3:** "Earth-League" candidate selection routine

**Data:** $CDHS$ score of a planet

**Result:** The habitability class of a planet

$k :=$ desired number of nearest neighbors to be considered;
$S := p_i, ..., p_n$, where $p_i = (x_i, c_i)$ is the $i^{th}$ training sample;
$S' := p'_i, ..., p'_n$, where $p'_i$ is the $i^{th}$ test sample;
$N :=$ number of samples in the training data;
$n :=$ number of samples in the test data;
$boundary := 1$;
$threshold := 0.4$;
**for** $i = 1$ *to* $N$ **do**
  **if** $habitability_i$ $=$ *1* **then**
    prob($habitability_i$) = 'high';
  **else**
    prob($habitability_i$) = 'low';
**for** $i = 1$ *to* $n$ **do**
  **if** *prob(*$habitability_i$*)* $=$ *'high' and* $CDHS(x_i) - CDHS(earth) \leq boundary$ **then**
    $x_i \in Class6$;
  **else**
    compute distance $d(x', x)$ between $p'_i$ and all other $p \in S$;
    select the $k$ nearest points to $p'$ from the list computed above;
    assign $p'$ the most common class in the nearest $k$ samples;
return the computed classes for each test sample

# 5 TRAPPIST-1 system: classification outcome

The classification system with the XGBoost Classifier can be used to classify the planets in TRAPPIST-1 system as well. Here, we present the classification results of the planets.

We have excluded TRAPPIST-1 g from this list as it belongs to the class of hypopsychroplanets; there are

Table 3: Classifying the planets in TRAPPIST-1

| Planet Name | Actual Class | Predicted Class |
|---|---|---|
| TRAPPIST-1 b | Non Habitable | Non Habitable |
| TRAPPIST-1 c | Non Habitable | Non Habitable |
| TRAPPIST-1 d | Mesoplanet | Mesoplanet |
| TRAPPIST-1 e | Psychroplanet | Psychroplanet |
| TRAPPIST-1 f | Psychroplanet | Psychroplanet |
| TRAPPIST-1 g | Psychroplanet | Psychroplanet |
| TRAPPIST-1 h | Non Habitable | Non Habitable |

not enough hypopsychroplanet samples in the dataset for a classification to be effective for TRAPPIST-1 g. The remaining samples have been classified using our system, and the predicted class labels for each test sample has been presented in Table 3.

# 6 XGBoost: An Exploration of Machine Learning based Classification

Boosting refers to the method of combining the results from a set of *weak learners* to produce a *strong* prediction. Generally, a weak learner's performance is close to a random guess. A *boosted* learner divides the job of a single predictor across many weak predictor functions, and optimally combines the votes from all smaller predictors. This helps enhancing the overall prediction accuracy.

XGBoost is a tool developed by utilizing these boosting principles [2]. XGBoost constructs trees by combining a large number of regressor functions with a small learning rate. As regression can be used to model classifiers, here the word *regression* may refer to logistic or soft-max regression for the task of classification. XGBoost uses an ensemble of decision trees. The boosting method used in XGBoost considers the functions added early to be significant, and the ones added later to be inconsequential. The major departure from random forests lies in how the trees are trained: XGBoost uses *gradient boosting.* Similar in nature to Random Forests, here an objective function is minimized while growing each tree, and each leaf has an associated score which determines the class membership of any test entity. The steps in XGBoost trees are as follows,

**Step 1**: Sample with replacement, $n$ training samples $X_b$, $Y_b$ from $X, Y$.

**Step 2**: A decision or tree is trained using multiple regressors $f_i$ on $X_b$, $Y_b$. An objective function is optimized while fitting the regressor.

**Step 3**: Step 2 is repeated until the all the samples in a given node is can be reliably approximated using the sum of all regressor functions (this is the paradigm of additive learning).

**Step 4**: Once this is complete, the best split is determined by calculating the gradient statistics and the Gain.

**Step 5**: Steps 2-4 are repeated by considering more trees. The results from each tree may be considered for the final classification in a majority-voting scheme.

**Step 6**: Once the model is trained, unobserved data is fed to it for classification.

Having described the idea of the data and the algorithm, we now proceed to the detailed description of the working principle of the algorithm.

## 6.1 Working Principles of XGBoost and an Example

XGBoosted Trees [2] may be understood by considering four central concepts [2]

[2]A part of this exploration may be found as a technical report on Research Gate: A Comparative Study in Classification Methods of Exoplanets Machine Learning Exploration via Mining and Automatic Labeling of the Habitability Catalog

### 6.1.1 Additive Learning

For additive learning, a set of regressor functions $f_i$ must be learned which estimate the distribution of data in each node of the tree. This is more difficult compared to traditional optimization problems, as there are multiple functions to be considered and it is not sufficient to optimize every tree by considering its gradient. Another overhead is with respect to implementation in a computer – it is difficult to estimate all the regressors at once. Thus, the training phase is divided into a sequence of steps. For $t$ steps, the prediction value from each step, $\hat{y}_i^{(t)}$, is added as:

$$\begin{aligned}
\hat{y}_i^{(0)} &= 0\,,\\
\hat{y}_i^{(1)} &= f_1(x_i) = \hat{y}_i^{(0)} + f_1(x_i)\,,\\
\hat{y}_i^{(2)} &= f_1(x_i) + f_2(x_i) = \hat{y}_i^{(1)} + f_2(x_i)\,,\\
&\dots\\
\hat{y}_i^{(t)} &= \sum_{k=1}^{t} f_k(x_i) = \hat{y}_i^{(t-1)} + f_t(x_i)\,. \qquad (14)
\end{aligned}$$

Central to any optimization method is an objective function which needs to be optimized. In each step, the regressor function must optimize the objective function of the learning algorithm. The objective function is formulated as:

$$\begin{aligned}
\text{obj}^{(t)} &= \sum_{i=1}^{n} l\left(y_i, \hat{y}_i^{(t)}\right) + \sum_{i=1}^{t} \Omega(f_i)\\
&= \sum_{i=1}^{n} l\left(y_i, \hat{y}_i^{(t-1)} + f_t(x_i)\right) + \Omega(f_t) + \text{constant}\,.
\end{aligned} \qquad (15)$$

Mean squared error (MSE) is used as its mathematical formulation is convenient, whereas e.g. logistic loss has a more complicated form. Since the error needs to be minimized, the gradient of the error must be calculated; for MSE, calculating the gradient and finding a minima is not difficult, but in the case of logistic loss, the process becomes more cumbersome. In the general case, Taylor expansion of the loss function is considered up to the term of a second order,

$$\begin{aligned}
\text{obj}^{(t)} \quad &= \quad \sum_{i=1}^{n} \left[ l(y_i, \hat{y}_i^{(t-1)}) + g_i f_t(x_i) + \frac{1}{2} h_i f_t^2(x_i) \right]\\
&+ \quad \Omega(f_t) + \text{constant}\,,
\end{aligned} \qquad (16)$$

where $g_i$ and $h_i$ are defined as:

$$\begin{aligned}
g_i &= \partial_{\hat{y}_i^{(t-1)}} l\left(y_i, \hat{y}_i^{(t-1)}\right)\\
h_i &= \partial^2_{\hat{y}_i^{(t-1)}} l\left(y_i, \hat{y}_i^{(t-1)}\right)
\end{aligned} \qquad (17)$$

By removing the lower order terms from Eq. (16), the objective function becomes

$$\sum_{i=1}^{n} \left[ g_i f_t(x_i) + \frac{1}{2} h_i f_t^2(x_i) \right] + \Omega(f_t)\,, \qquad (18)$$

which is the optimization equation of XGBoost.

### 6.1.2 Model Complexity and Regularized Learning Objective

The definition of the tree $f(x)$ may be refined as

$$f_t(x) = w_{q(x)}\,, \quad w \in R^T,\ q : R^d \to \{1, 2, \dots, T\}\,, \qquad (19)$$

where $w$ is the vector of scores on leaves, $q$ is a function assigning each data point to the corresponding leaf, and $T$ is the number of leaves. The model complexity in XGBoost may be given as:

$$\Omega(f) = \gamma T + \frac{1}{2} \lambda \sum_{j=1}^{T} w_j^2\,. \qquad (20)$$

A regularized objective is minimized for the algorithm to learn the set of functions given in the model. It is given by

$$\mathcal{L}(\phi) = \sum_i l(\hat{y}_i, y_i) + \sum_k \Omega(f_k)\,. \tag{21}$$

### 6.1.3 Structure Score

After the objective value has been re-formalized, the objective value of the $t^{th}$ tree may be calculated as

$$\begin{aligned} Obj^{(t)} &\approx \sum_{i=1}^{n} \left[ g_i w_{q(x_i)} + \frac{1}{2} h_i w_{q(x_i)}^2 \right] + \gamma T + \frac{1}{2}\lambda \sum_{j=1}^{T} w_j^2 \\ &= \sum_{j=1}^{T} \left[ \left( \sum_{i \in I_j} g_i \right) w_j + \frac{1}{2} \left( \sum_{i \in I_j} h_i + \lambda \right) w_j^2 \right] + \gamma T\,, \end{aligned} \tag{22}$$

where $I_j = \{i|q(x_i) = j\}$ is the set of indices of data points assigned to the $j^{th}$ leaf.

In the second line of Eq. (22), the index of the summation has been changed because all the data points in the same leaf must have the same score. Let $G_j = \sum_{i \in I_j} g_i$ and $H_j = \sum_{i \in I_j} h_i$. The equation can be rewritten by substituting for $G$ and $H$ as

$$\text{Obj}^{(t)} = \sum_{j=1}^{T} \left[ G_j w_j + \frac{1}{2}(H_j + \lambda) w_j^2 \right] + \gamma T\,. \tag{23}$$

In Eq. (23), every $w_j$ is independent of each other. The form $G_j w_j + \frac{1}{2}(H_j + \lambda)w_j^2$ is quadratic, and the best $w_j$ for a given structure $q(x)$ and the best objective reduction which measures goodness of tree is

$$w_j^* = -\frac{G_j}{H_j + \lambda} \text{Obj}^* = -\frac{1}{2} \sum_{j=1}^{T} \frac{G_j^2}{H_j + \lambda} + \gamma T\,. \tag{24}$$

### 6.1.4 Learning Structure Score

**XGBoost learns the tree level based on the following equation**

$$Gain = \frac{1}{2} \left[ \frac{G_L^2}{H_L + \lambda} + \frac{G_R^2}{H_R + \lambda} - \frac{(G_L + G_R)^2}{H_L + H_R + \lambda} \right] - \gamma. \tag{25}$$

The equation comprises four main parts:

- The score on the new left leaf,
- The score on the new right leaf,
- The score on the original leaf,
- Regularization on the additional leaf.

The value of *Gain* should as high as possible for learning to take place effectively. Hence, if the value of *Gain* is greater than $\gamma$, the corresponding branch should not be added.

## 6.2 An Example

Both Random Forests and XGBoosted trees are built using an ensemble of trees. The key difference between these methods lies in how the trees are constructed and trained. Having explained the mathematical formulation of formation of XGBoosted trees, we proceed to discuss the following illustrative example.

Let us consider three attributes it S.HabCat, P.Ts Min, P.Surf.Pres, and eight entities which are used for training. The class labels, corresponding values for attributes, and gradient statistics are given in Table 4.

Using these entities, a tree is constructed, as shown in Figs. 1 and 2.

Using index $I$, and statistics $G$ and $H$, the scores for each leaf node may be calculated as:

Table 4: Set of Entities for Illustrative Examples

| No. | Class | S.HabCat | P.Ts Min | P.Surf.Pres. | Grad. Stats |
|---|---|---|---|---|---|
| 1 | N-H | 1 | 476.1 | 1.8 | g1, h1 |
| 2 | N-H | 1 | 690.7 | 4.8 | g2, h2 |
| 3 | N-H | 0 | 916.1 | 15.1 | g3, h3 |
| 4 | N-H | 0 | 916.1 | 2870.4 | g4, h4 |
| 5 | P | 0 | 262.8 | 8.6 | g5, h5 |
| 6 | P | 0 | 225.2 | 2.7 | g6, h6 |
| 7 | M | 0 | 298.4 | 10.2 | g7, h7 |
| 8 | M | 0 | 270.6 | 12.6 | g8, h8 |

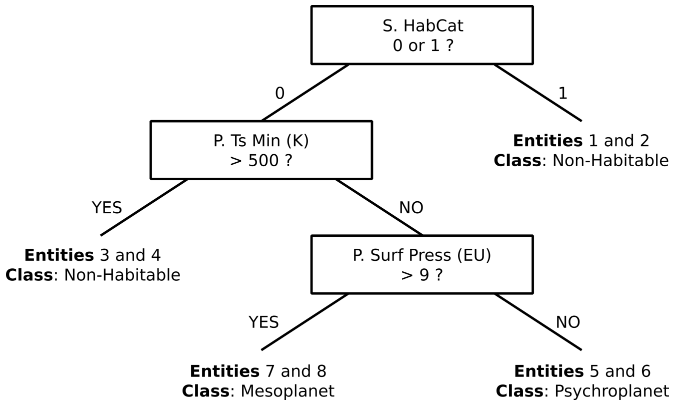


Figure 1: An example XGBoosted Tree

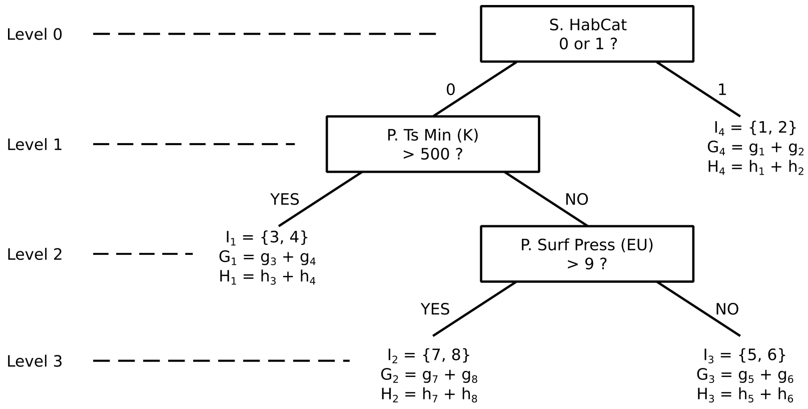


Figure 2: Calculating Gradient Statistics

$$
\begin{aligned}
G_1 &= g_3 + g_4 & H_1 &= h_3 + h_4 \\
G_2 &= g_7 + g_8 & H_2 &= h_7 + h_8 \\
G_3 &= g_5 + g_6 & H_3 &= h_5 + h_6 \\
G_4 &= g_1 + g_2 & H_4 &= h_1 + h_2
\end{aligned} \tag{26}
$$

The score is an indicator of how good a tree is (Section 6.1.3).

The next step is to select the best tree based on the structure score. *Gain* is calculated at each level at each branch of the tree. Calculating *Gain* is an intractable problem; it is hence calculated at each level, following a divide-and-conquer ideology. *Gain* calculated at level 1 for the right branch in the tree given in Fig. 2 is

$$
Obj = \frac{-G_4}{H_4 + \lambda} + \gamma\,. \tag{27}
$$

For *Gain* to be calculated at level 2,

$$
Obj = -\sum_{j=2,3} \frac{-G_j}{H_j + \lambda} + 2\gamma\,. \tag{28}
$$

Similarly, *Gain* is calculated for each branch. If *Gain* is smaller than $\gamma$ for any branch, it is best not to add that branch. Thus, this method is how XGBoosted trees are pruned.

# References


[1] Saha S., Sarkar J., Dwivedi A., Dwivedi N., Anand M. N., Roy R., 2016. A novel revenue optimization model to address the operation and maintenance cost of a data center. *Journal of Cloud Computing*, 5:1, 1-23.

[2] Chen T., Guestrin C., XGBoost: A Scalable Tree Boosting System, Preprint arXiv:1603.02754
